# Supplementary material for: Exactly Computing the Local Lipschitz Constant of ReLU Networks
Source: arXiv:2003.01219 source file (2021-01-11)
Supplement: Supplementary file 2 [file app_main.tex]

\documentclass{article}

% Recommended, but optional, packages for figures and better typesetting:
\usepackage{microtype}
\usepackage{graphicx}
\usepackage{subfig}
\usepackage{booktabs} % for professional tables
\usepackage{amsmath}
\usepackage{amssymb}
\usepackage{amsthm}

\usepackage[numbers, square, comma, compress, sort]{natbib}

\setcounter{tocdepth}{2}
\usepackage[shortlabels]{enumitem}
% X => Y

% hyperref makes hyperlinks in the resulting PDF.
% If your build breaks (sometimes temporarily if a hyperlink spans a page)
% please comment out the following usepackage line and replace
% \usepackage{icml2019} with \usepackage[nohyperref]{icml2019} above.
\usepackage{hyperref}

% Attempt to make hyperref and algorithmic work together better:

% Use the following line for the initial blind version submitted for review:

\usepackage{appstyle}

% If accepted, instead use the following line for the camera-ready submission:
%\usepackage[accepted]{icml2019}

% The \icmltitle you define below is probably too long as a header.
% Therefore, a short form for the running title is supplied here:
\icmltitlerunning{Appendices}
\pagenumbering{arabic}
\bibliographystyle{unsrtnat}

\begin{document}

\onecolumn

\icmltitle{Appendices}
Contained in the supplementary are several standalone components. We have tried to include all relevant preliminary information where applicable. The proof of Theorem 1 is contained in Appendix A. The proofs of the statements in section 3 of the main paper are contained in Appendix B. The inapproximability results are presented in Appendix C. The formal construction and bound-propagation schemes of LipMIP are contained in Appendix D. Extension of LipMIP to general position vector-valued networks over a wider class of norms is contained in Appendix E. Appendix F has full experimental details and additional experiments.
\tableofcontents
\newpage
% APPENDIX OUTLINE 
% Analytical results

% Section 1: Proofs for analysis sections 
\input{appendices/app_1_analysis}
% Section 2: Proofs for General Position section 
\input{appendices/app_2_gp}
% Section 3: Proofs for inapproximability 
\input{appendices/app_3_inapprox}
% Section 4: Proofs for LipMIP
% Construction of LipMIP
% -- ACS of Neural networks 
% -- ACS MIP-encodability 
% -- Abstract Interpretation 
\input{appendices/app_4_lipmip1}

% Section 5: Extensions to LipMIP 
\input{appendices/app_5_extensions}
% Section 6: Extra experiments 
\input{appendices/app_6_experiments}
\bibliography{appendices/app_bib}

\end{document}
